# Supplementary material for: Quantum spin Hall effect in two-dimensional transition-metal chalcogenides
Source: arXiv:2109.01209 source file (2021-09-30)
Supplement: Supplementary file 1 [file SupplementalMaterial.pdf]

## SUPPLEMENTAL MATERIAL

# Quantum spin Hall effect in two-dimensional transition-metal chalcogenides

Xing Wang,[1,2] Wenhui Wan,[1] Yanfeng Ge,[1] Kai-Cheng Zhang,[3] and Yong Liu[1,*]

[1]*State Key Laboratory of Metastable Materials Science and Technology & Key Laboratory for Microstructural Material Physics of Hebei Province, School of Science, Yanshan University, Qinhuangdao 066004, China*

[2]*College of Science, Hebei North University, Zhangjiakou 07500, China*

[3]*College of Mathematics and Physics, Bohai University, Jinzhou 121013, China*

(Dated: September 26, 2021)

This Supplemental Material is meant to support the explanations described in the main text entitled ”Quantum spin Hall effect in two-dimensional transition-metal chalcogenides”.

Part I The crystal orbital Hamilton population (COHP) curves of single-layer $ZrSe_5$ and $ZrTe_5$.

Part II The molecular dynamics (MD) simulation for single-layer $ZrSe_5$ and $ZrTe_5$.

Part III Electron localization function (ELF), difference charge density of single-layer $ZrSe_5$.

Part IV Electron localization function (ELF), difference charge density of single-layer $ZrTe_5$.

Part V The total density of states (DOS) and projected density of states (PDOS) for single-layer $ZrSe_5$ and $ZrTe_5$.

Part VI The band structures of single-layer $ZrSe_5$ and $ZrTe_5$.

Part VII The evolution of Wannier charge centers of single-layer $ZrSe_5$ and $ZrTe_5$.

Part VIII The edge states of single-layer $ZrSe_5$ and $ZrTe_5$.

Part IX The molecular dynamics simulation for single-layer $HfX_5$.

Part X The band structures of single-layer $HfX_5$.

## Part I The crystal orbital Hamilton population (COHP) curves of single-layer $ZrSe_5$ and $ZrTe_5$.

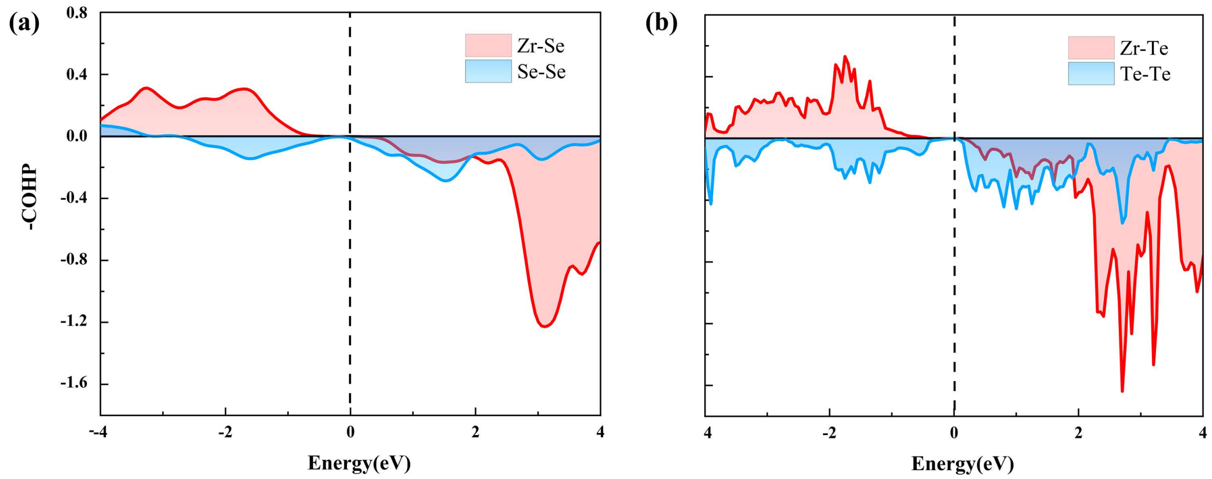


FIG. S1. (Color online) The crystal orbital Hamilton population (COHP) curves of single-layer (a) $ZrSe_5$ and (b) $ZrTe_5$. The Fermi levels are marked by the vertical dashed lines.


* yongliu@ysu.edu.cn or ycliu@ysu.edu.cn

Part II The molecular dynamics (MD) simulation for single-layer $ZrSe_5$ and $ZrTe_5$.

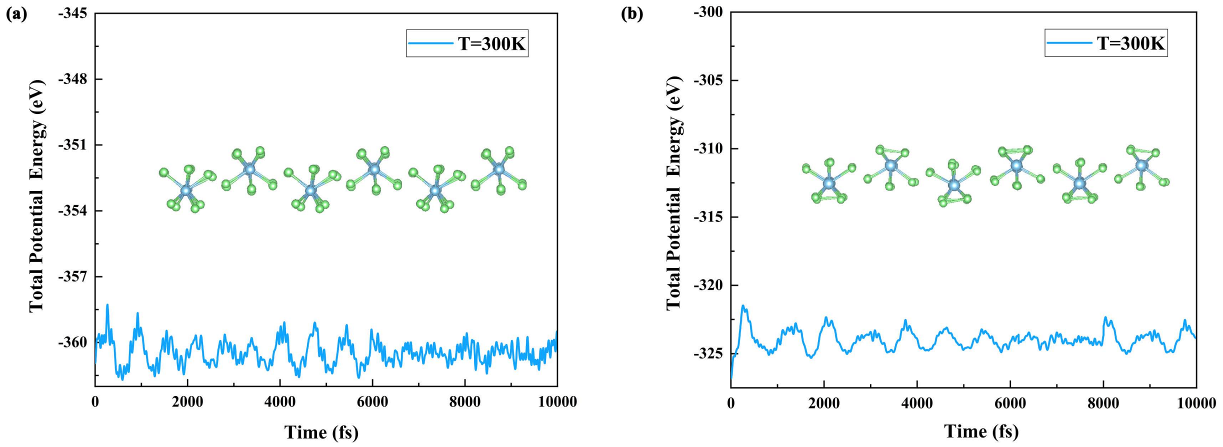


FIG. S2. (Color online) The snapshots of atomic configurations at the end of MD simulation and total potential energy fluctuations observed at 300K of single-layer (a) $ZrSe_5$ and (b) $ZrTe_5$.

Part III Electron localization function (ELF), difference charge density of single-layer $ZrSe_5$.

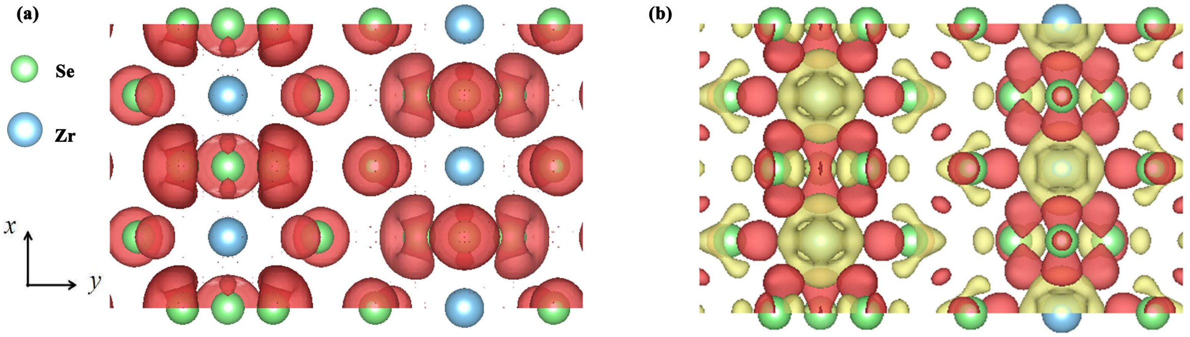


FIG. S3. (Color online) Electron localization function (ELF), difference charge density of single-layer $ZrSe_5$. (a) Structure plot of ELF. Isosurface corresponding to ELF value of 0.85. (b) Difference charge density (crystal density minus superposition of isolated atomic densities). The red (yellow) isosurface plots correspond to the charge density accumulation (depletion).

Part IV Electron localization function (ELF), difference charge density of single-layer $ZrTe_5$.

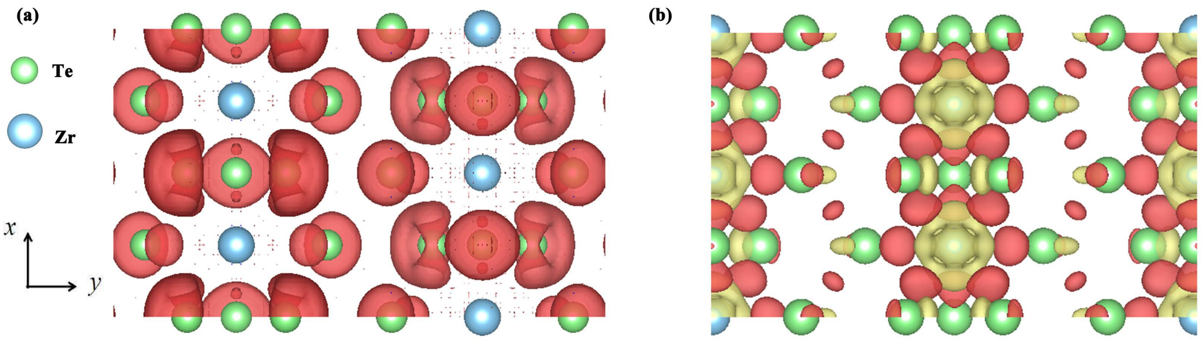


FIG. S4. (Color online) Electron localization function (ELF), difference charge density of single-layer $ZrTe_5$. (a) Structure plot of ELF. Isosurface corresponding to ELF value of 0.85. (b) Difference charge density. The red (yellow) isosurface plots correspond to the charge density accumulation (depletion).

Part V The total density of states (DOS) and projected density of states (PDOS) for single-layer $ZrSe_5$ and $ZrTe_5$.

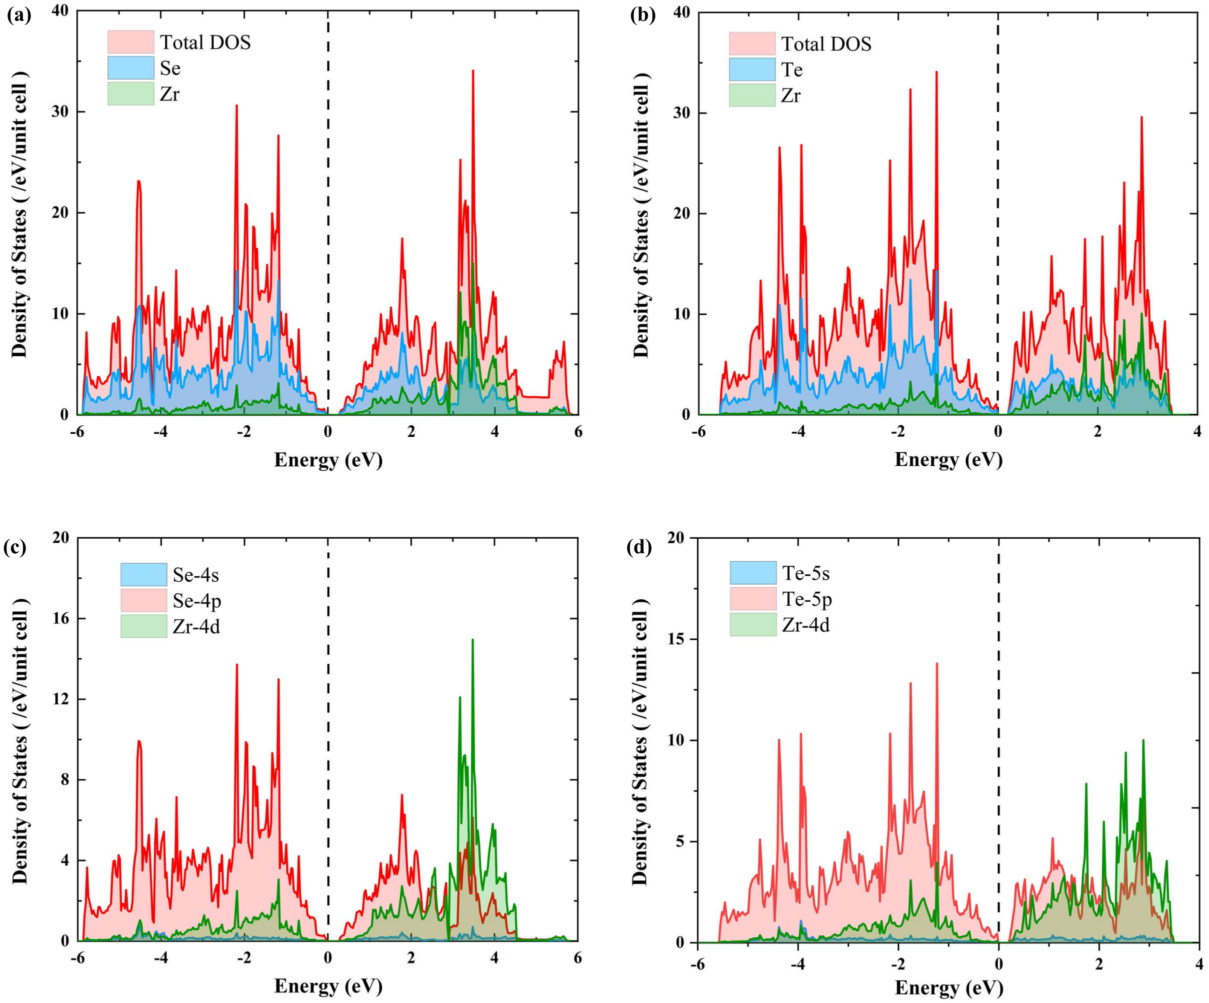


FIG. S5. (Color online) The total density of states (DOS) and projected density of states (PDOS) with consideration of SOC for single-layer (a, c) $ZrSe_5$ and (b, d) $ZrTe_5$. The Fermi levels are set to zero and marked by short dash lines.

Part VI The band structures of single-layer $ZrSe_5$ and $ZrTe_5$.

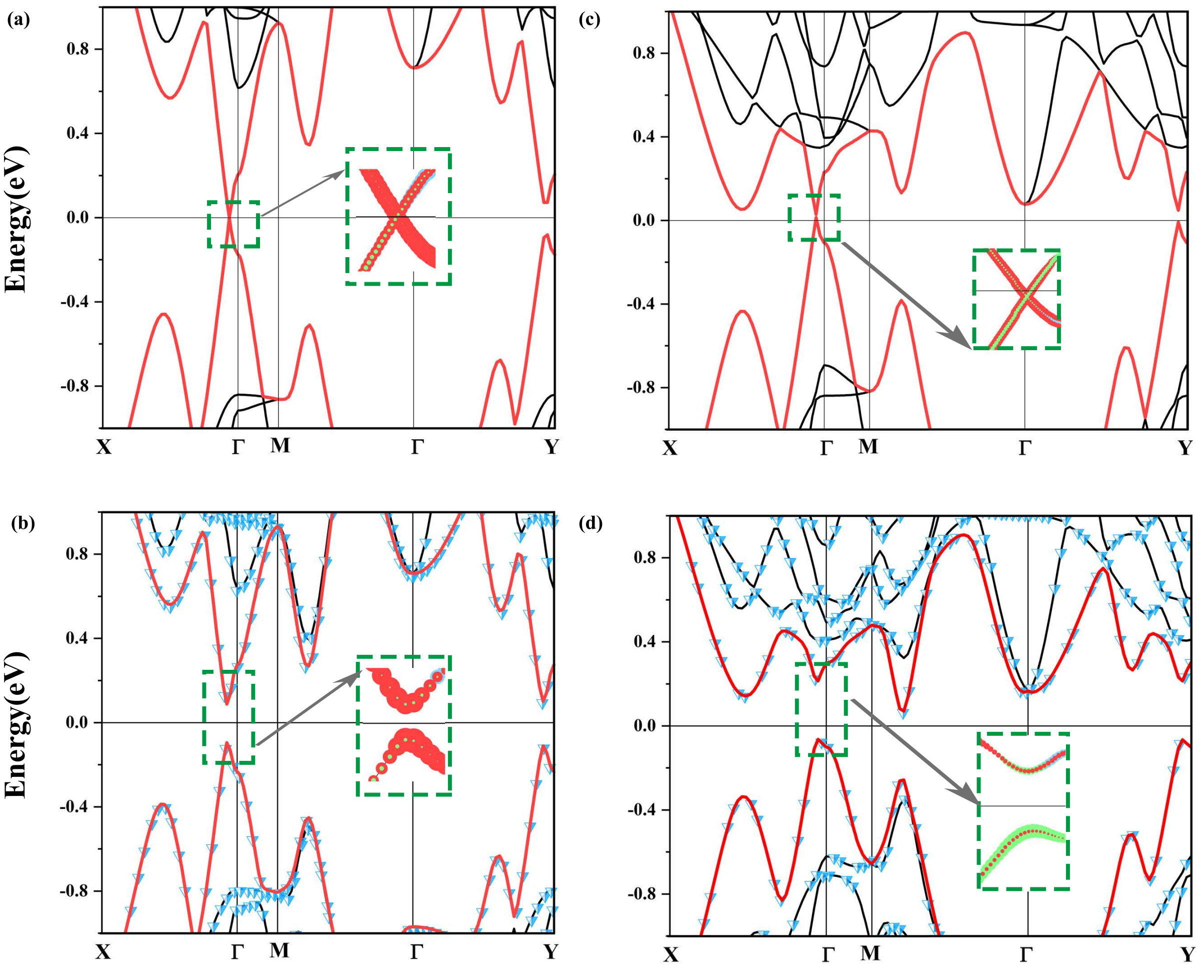


FIG. S6. (Color online) The band structures of single-layer $ZrSe_5$ and $ZrTe_5$ for (a, c) without and (b, d) with SOC, respectively. The blue triangles indicate the band structures diagrams calculated by Wannier90. The enlarged orbitals-resolved band structures are shown in insets. The green and red circles represent the weights of the Se1-4p (or Te1-5p) and Se2-4p (or Te2-5p) character, respectively. The Fermi levels are set to zero.

Part VII The evolution of Wannier charge centers of single-layer $ZrSe_5$ and $ZrTe_5$.

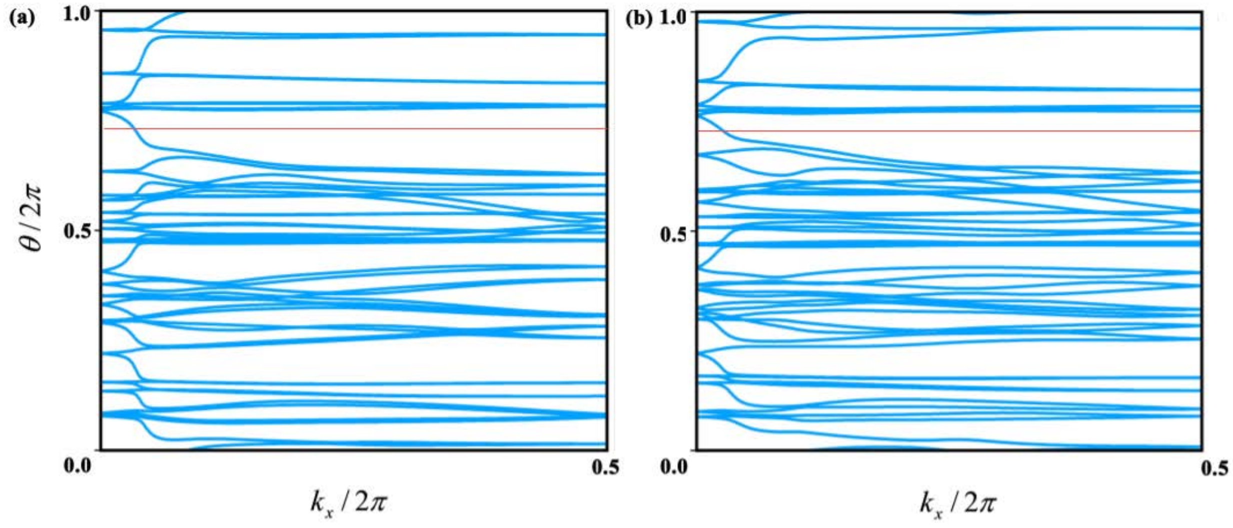


FIG. S7. (Color online) The evolution of Wannier charge centers of single-layer (a) $ZrSe_5$ and (b) $ZrTe_5$. The evolution of Wannier charge centers along $k_x$. The evolution blue lines cross the arbitrary reference red line one time yielding $Z_2$=1.

Part VIII The edge states of single-layer $ZrSe_5$ and $ZrTe_5$.

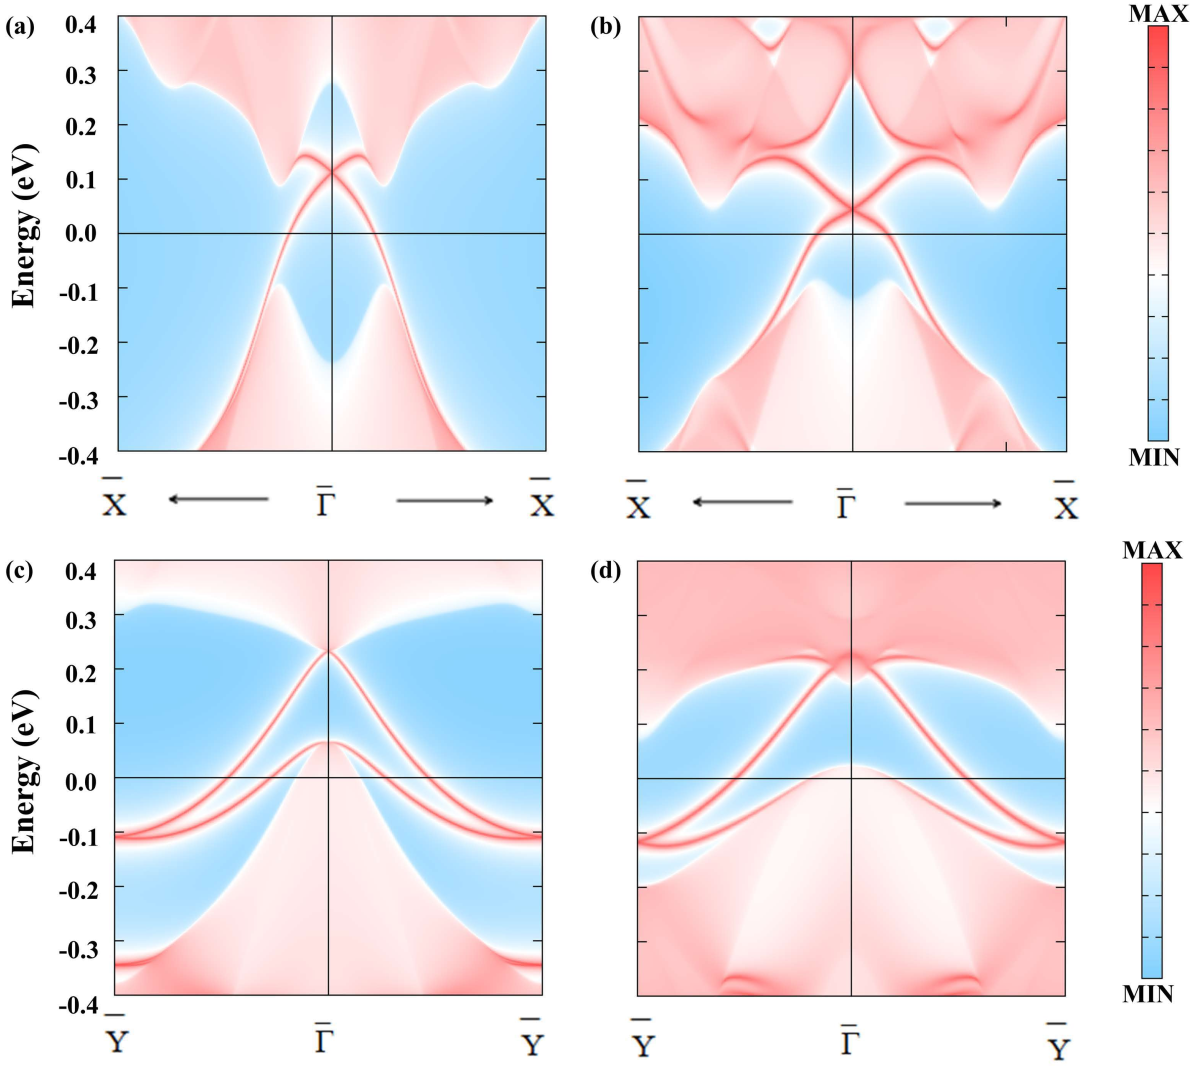


FIG. S8. (Color online) The edge states of single-layer (a, c) $ZrSe_5$ and (b, d) $ZrTe_5$. The edge state for (a, b) *x* edge and (c, d) *y* edge.

Part IX The molecular dynamics simulation for single-layer $HfX_5$.

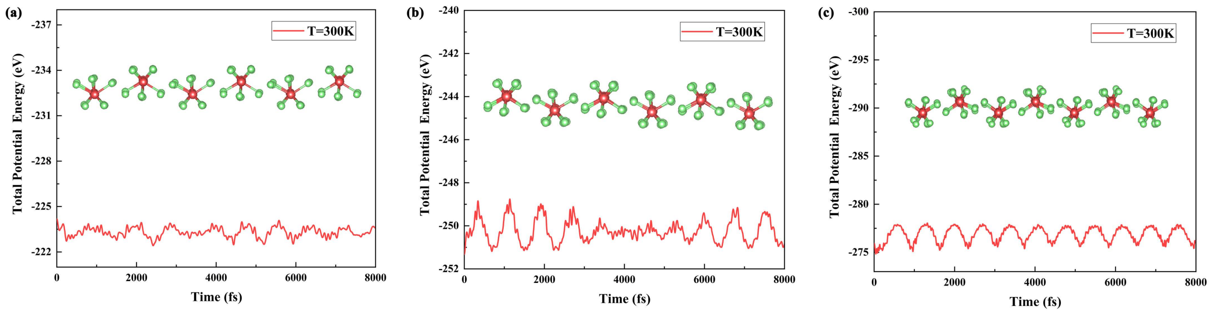


FIG. S9. (Color online) Snapshots of atomic configurations at the end of MD simulation and total potential energy fluctuations observed at 300K of single-layer (a) $HfTe_5$ , (b)$HfSe_5$ and (c) $HfS_5$, respectively.

Part X The band structures of single-layer $HfX_5$.

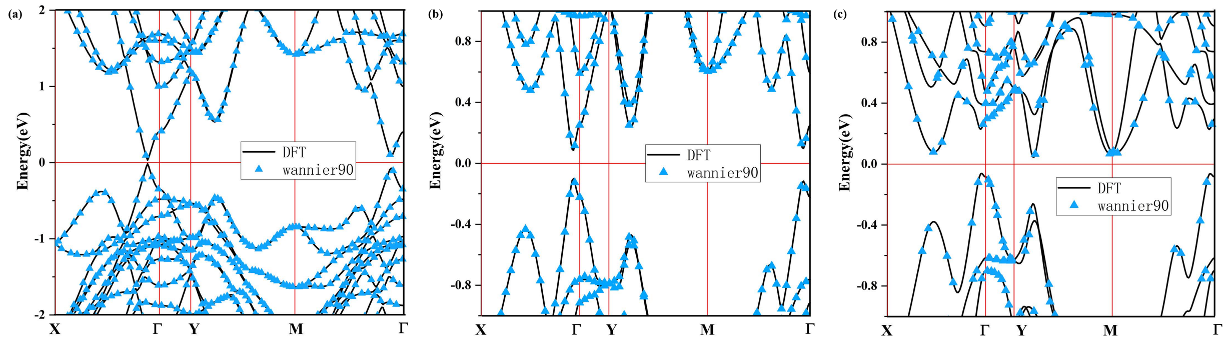


FIG. S10. (Color online) The band structures of single-layer (a) $HfS_5$ , (b)$HfSe_5$ and (c) $HfTe_5$ with SOC, respectively. The blue triangles indicate the band structures diagrams calculated by Wannier90. The Fermi levels are set to zero.
